# Supplementary material for: AI Greenferencing: Routing AI Inferencing to Green Modular Data Centers with Heron
Source: arXiv:2505.09989 source file (2025-05-15)
Supplement: Supplementary file 1 [file appendix.tex]

\section{Appendix}
\label{appendix}
